# Supplementary material for: Learning to Balance: Bayesian Meta-Learning for Imbalanced and Out-of-distribution Tasks
Source: arXiv:1905.12917 source file (2022-02-12)
Supplement: Supplementary file 1 [file bayesian_table_appendix.tex]

\begin{table*}[h]
	\begin{center}
			\begin{tabular}{ccc}
				\toprule
				Models ($K$=5) & Omniglot & MNIST\\
				\hline
				\hline
				MAML						& 98.32 $\pm$ 0.26 & 89.19 $\pm$ 0.31	\\
				Meta-SGD 					& 98.38 $\pm$ 0.23 & 90.42 $\pm$ 0.28	\\
				ABML						& 98.67 $\pm$ 0.30 & 90.69 $\pm$ 0.34	\\
				\hline
				Deterministic TAML 			& 98.75 $\pm$ 0.34 & 90.77 $\pm$ 0.36	\\
				%Bayesian $g(\bz^\ts)$ TAML	& \bf98.92 & \bf92.06	\\
				Bayesian TAML				& \bf99.13 $\pm$ 0.31& \bf92.38 $\pm$ 0.33	\\
				\bottomrule
		\end{tabular}
		\label{tbl:bayesian_appendix}
\vspace{-0.15in}
\end{center}
\caption{\small Distribution discrepancy results.}
\end{table*}
