# Supplementary material for: Learning to Balance: Bayesian Meta-Learning for Imbalanced and Out-of-distribution Tasks
Source: arXiv:1905.12917 source file (2022-02-12)
Supplement: Supplementary file 2 [file cimbal_table_appendix.tex]

\begin{table*}[!h]
	\begin{center}
		\begin{tabular}{cccc}
			\toprule
			Models ($K$=5) & x1 & x5 & x15\\
			\hline
			\hline
			MAML		& \bf98.17 $\pm$ 0.35 & 95.77 $\pm$ 0.42	& 84.97 $\pm$ 0.51	\\
			Meta-SGD 	& 97.31 $\pm$ 0.33 & 95.38 $\pm$ 0.38 & 89.12 $\pm$ 0.47	\\
			ABML		& 97.79 $\pm$ 0.37 & 95.89 $\pm$ 0.41 & 91.09 $\pm$ 0.52	\\
			\hline
			Bayesian $g(\bs\omega^\ts)$ TAML 	& 97.29 $\pm$ 0.37 & \bf96.82 $\pm$ 0.44	& \bf91.61 $\pm$ 0.53	\\
			\bottomrule
		\end{tabular}
		\label{tbl:cimbal_appendix}
		\vspace{-0.15in}
	\end{center}
\caption{\small Class-Imbalance results.}
\end{table*}
