# Supplementary material for: Learning to Balance: Bayesian Meta-Learning for Imbalanced and Out-of-distribution Tasks
Source: arXiv:1905.12917 source file (2022-02-12)
Supplement: Supplementary file 3 [file ood_table_appendix.tex]

\begin{table*}[h]
	\begin{center}
		\begin{tabular}{ccc}
			\toprule
			Models ($K$=5) & Omniglot & MNIST\\
			\hline
			\hline
			MAML						& 98.32 $\pm$ 0.26 & 89.19 $\pm$ 0.31	\\
			Meta-SGD 					& 98.38 $\pm$ 0.23 & 90.42 $\pm$ 0.28	\\
			ABML						& 98.67 $\pm$ 0.30 & 90.69 $\pm$ 0.34	\\
			\hline
			Bayesian $g(\bz^\ts)$ TAML	& \bf98.92 $\pm$ 0.30 & \bf92.06 $\pm$ 0.32	\\
			%Bayesian TAML				& \bf99.13 & \bf92.38	\\
			\bottomrule

		\end{tabular}		
\label{tbl:ood_appendix}
\vspace{-0.15in}
\end{center}
\caption{\small Distribution discrepancy results.}
\end{table*}
