# Supplementary material for: Learning to Balance: Bayesian Meta-Learning for Imbalanced and Out-of-distribution Tasks
Source: arXiv:1905.12917 source file (2022-02-12)
Supplement: Supplementary file 4 [file supplementary_table.tex]

\begin{table}[h]
	%\vspace{-0.1in}
	\small
	\begin{center}
		\begin{tabular}{ccc|cc}
			\toprule
			Models ($K$=5) 				 & Omniglot 				 & MNIST 					& tiered-ImageNet 			& mini-ImageNet\\
			\hline
			\hline
			Bayesian TAML (Naive approx.) & 96.18 	 \tiny$\pm$ 0.33 & 83.95    \tiny$\pm$ 0.52 & 71.17     \tiny$\pm$ 1.09 & 57.68    \tiny$\pm$ 0.48\\
			Bayesian TAML (MC approx.)	  & \bf96.29 \tiny$\pm$ 0.31 & \bf84.39 \tiny$\pm$ 0.48 & \bf 71.42 \tiny$\pm$ 1.00 & \bf58.37 \tiny$\pm$ 0.49\\
			\bottomrule
		\end{tabular}
	\end{center}
	\small
	\caption{\small \textbf{Classification performance under realistic scenario.} The models are trained with Omniglot(left) and tiered-ImageNet(right) with imbalanced setting. All reported results are average performances over 1000 for Omniglot and MNIST and 600 for tiered-ImageNet and mini-ImageNet randomly selected episodes with standard errors for 95\% confidence interval over tasks.}\label{tbl:analysis_spl}
	\vspace{-0.08in}
\end{table}
